# Supplementary material for: Persona is a Double-edged Sword: Mitigating the Negative Impact of Role-playing Prompts in Zero-shot Reasoning Tasks
Source: arXiv:2408.08631 source file (2024-10-19)
Supplement: Supplementary file 1 [file numdata_appendix.tex]

\begin{figure*}[h]
\centerline{\includegraphics[width=1.0\linewidth]{fig_files/numdata_appendix.pdf}}
\vspace{-0.2cm}
\caption{\textbf{Bias mitigation results for varying numbers of data samples to compute bias attribution.}
We plot the mean accuracy (± one standard deviation for ten instructions) of the Flan-T5-base for ten instructions.}
\label{numdata}
\end{figure*}
