# Supplementary material for: Persona is a Double-edged Sword: Mitigating the Negative Impact of Role-playing Prompts in Zero-shot Reasoning Tasks
Source: arXiv:2408.08631 source file (2024-10-19)
Supplement: Supplementary file 2 [file transfer_appendix.tex]

\begin{figure*}[h]
\centerline{\includegraphics[width=1.0\linewidth]{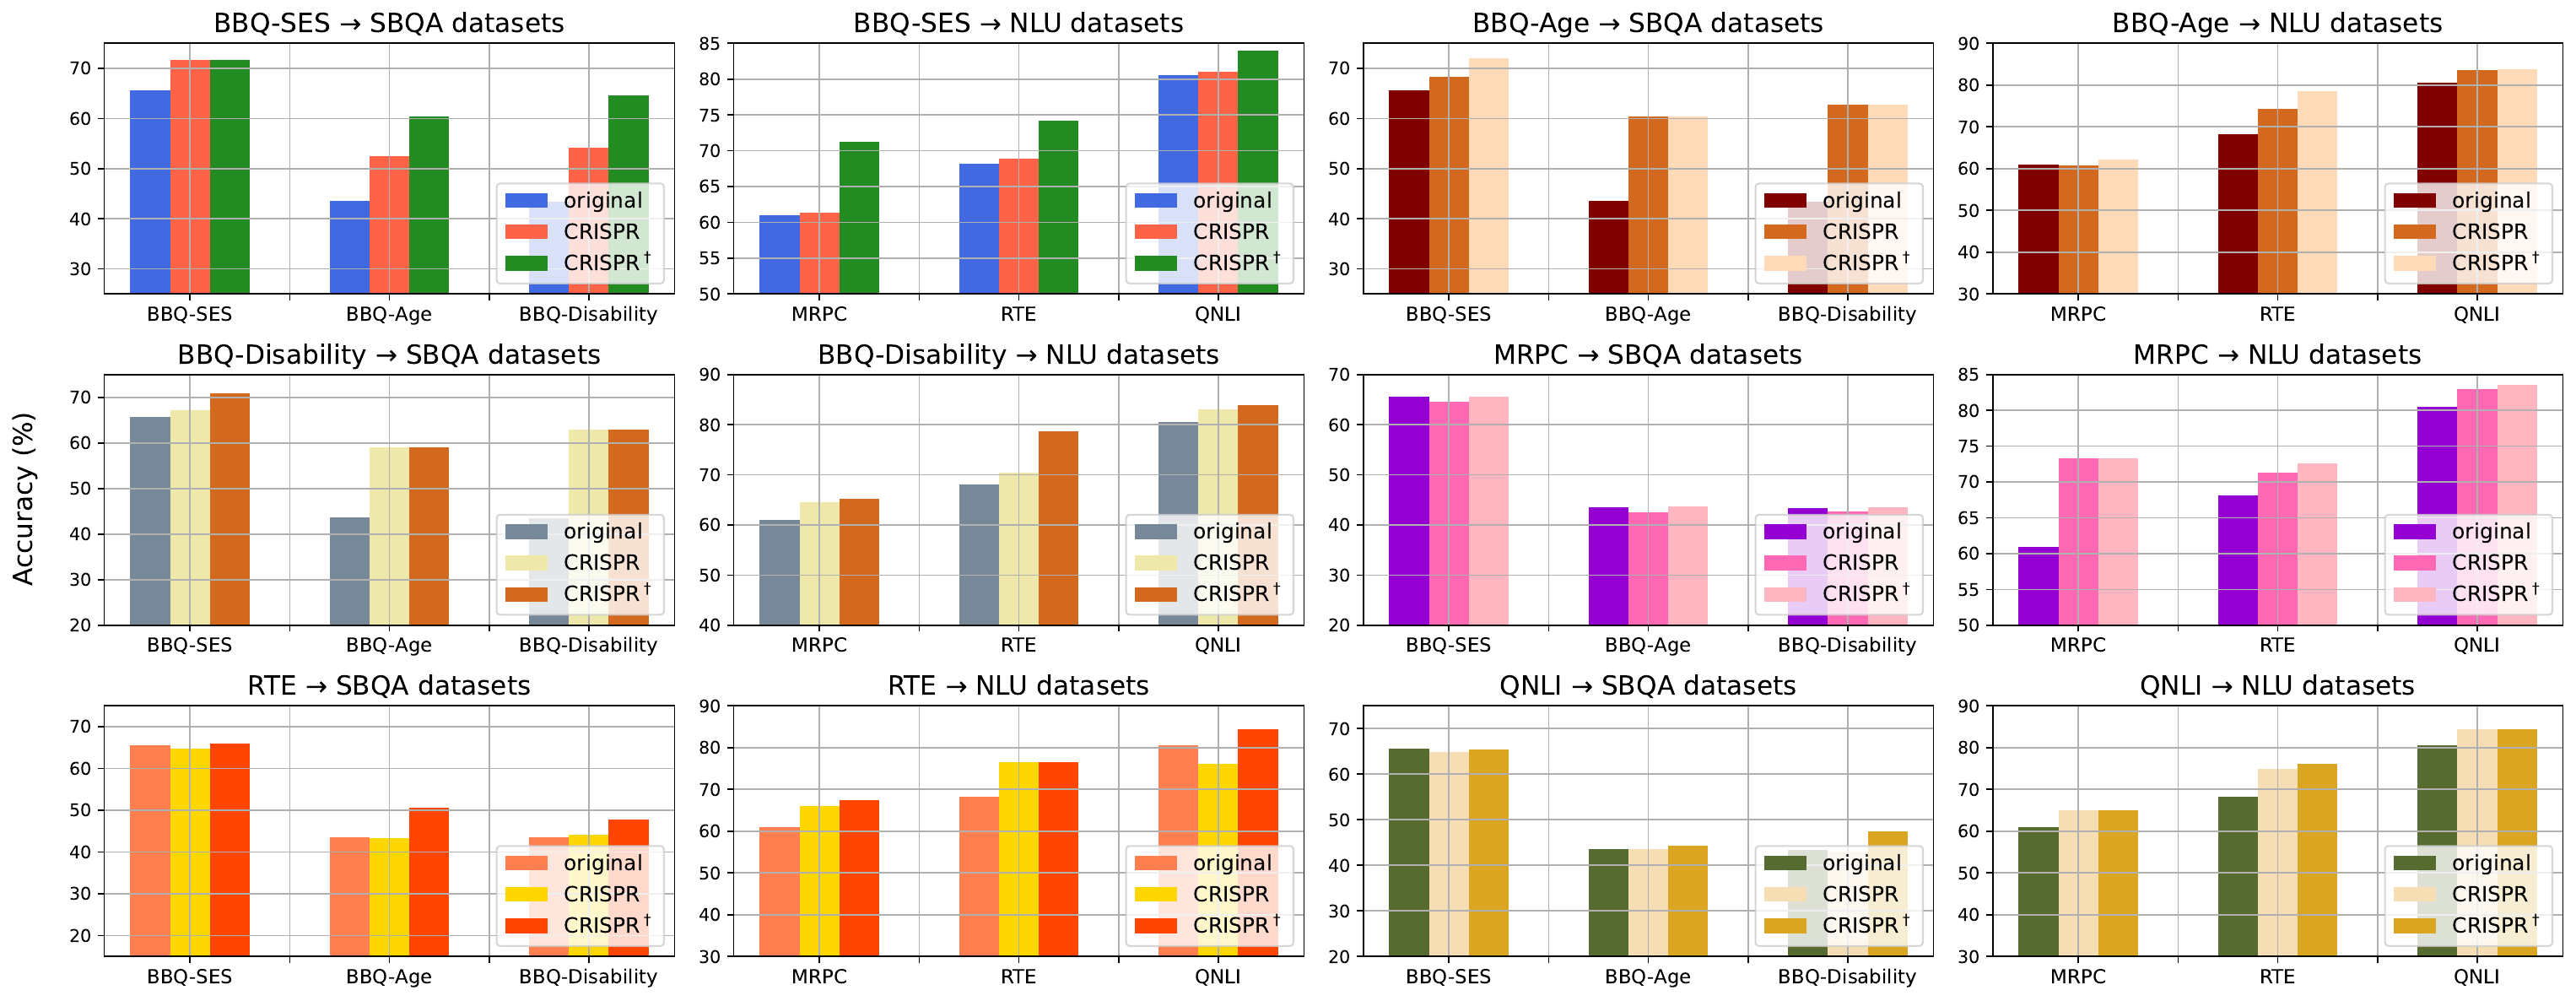}}
\vspace{-0.2cm}
\caption{\textbf{Skill Knowledge Preservation and Bias Knowledge Transfer Experiments}. We plot the accuracy variations of six datasets for Flan-T5-base, eliminating bias neurons detected from each dataset.
CRISPR determines the optimal number of bias neurons by measuring the acccuracy of the original attribution-computed datasets.
CRISPR$^\dagger$ searches the optimal number of bias neurons by measuring the accuracy of the each target evaluation dataset.}
\label{transfer_appendix}
\end{figure*}
